# Supplementary material for: Guiding Language Models of Code with Global Context using Monitors
Source: arXiv:2306.10763 source file (2023-11-03)
Supplement: Supplementary file 1 [file appendix_examples.pdf]

```
    }).collect(Collectors.toList());
    return ListResult.of(envVOS);
}
```

```
    getDesc());
    return envVO;
}).collect(Collectors.toList());
return ListResult.success(envVOS);
```

```
    getDescription());
    return envVO;
}).collect(Collectors.toList(
return ListResult.of(envVOS);
```

## Prompt

```java
public ListResult<EnvVO> list() {
    List<EnvVO> envVOS = Arrays.stream(
        EnvTypeEnum.values()).map(envTypeEnum -> {
        EnvVO envVO = new EnvVO();
        envVO.setCode(envTypeEnum.getCode());
        envVO.setName(envTypeEnum.
}
```

## Ground Truth

```java
            getDescription());
        return envVO;
    }).collect(Collectors.toList());
    return ListResult.of(envVOS);
}
```

## TD-3

```java
            getName());
        return envVO;
    }).collect(Collectors.toList());
    return ListResult.success(envVOS);
```

## SC

```java
            getDesc());
        return envVO;
    }).collect(Collectors.toList());
    return ListResult.success(envVOS);
}
```

## SC-MGD

```java
            getDescription());
        return envVO;
    }).collect(Collectors.toList());
    return ListResult.of(envVOS);
}
```

## Prompt

```java
public ListResult<EnvVO> list() {
    List<EnvVO> envVOS = Arrays.stream(
        EnvTypeEnum.values()).map(envTypeEnum -> {
        EnvVO envVO = new EnvVO();
        envVO.setCode(envTypeEnum.getCode());
        envVO.setName(envTypeEnum.
}
```

## Ground Truth

```java
        getDescription());
        return envVO;
    }).collect(Collectors.toList());
    return ListResult.of(envVOS);
}
```

```java
        getName());
        return envVO;
    }).collect(Collectors.toList());
    return ListResult.success(envVOS);
}
```

## SC

```java
        getDesc());
        return envVO;
    }).collect(Collectors.toList());
    return ListResult.success(envVOS);
}
```

## SC-MGD

```java
        getDescription());
        return envVO;
    }).collect(Collectors.toList());
    return ListResult.of(envVOS);
```

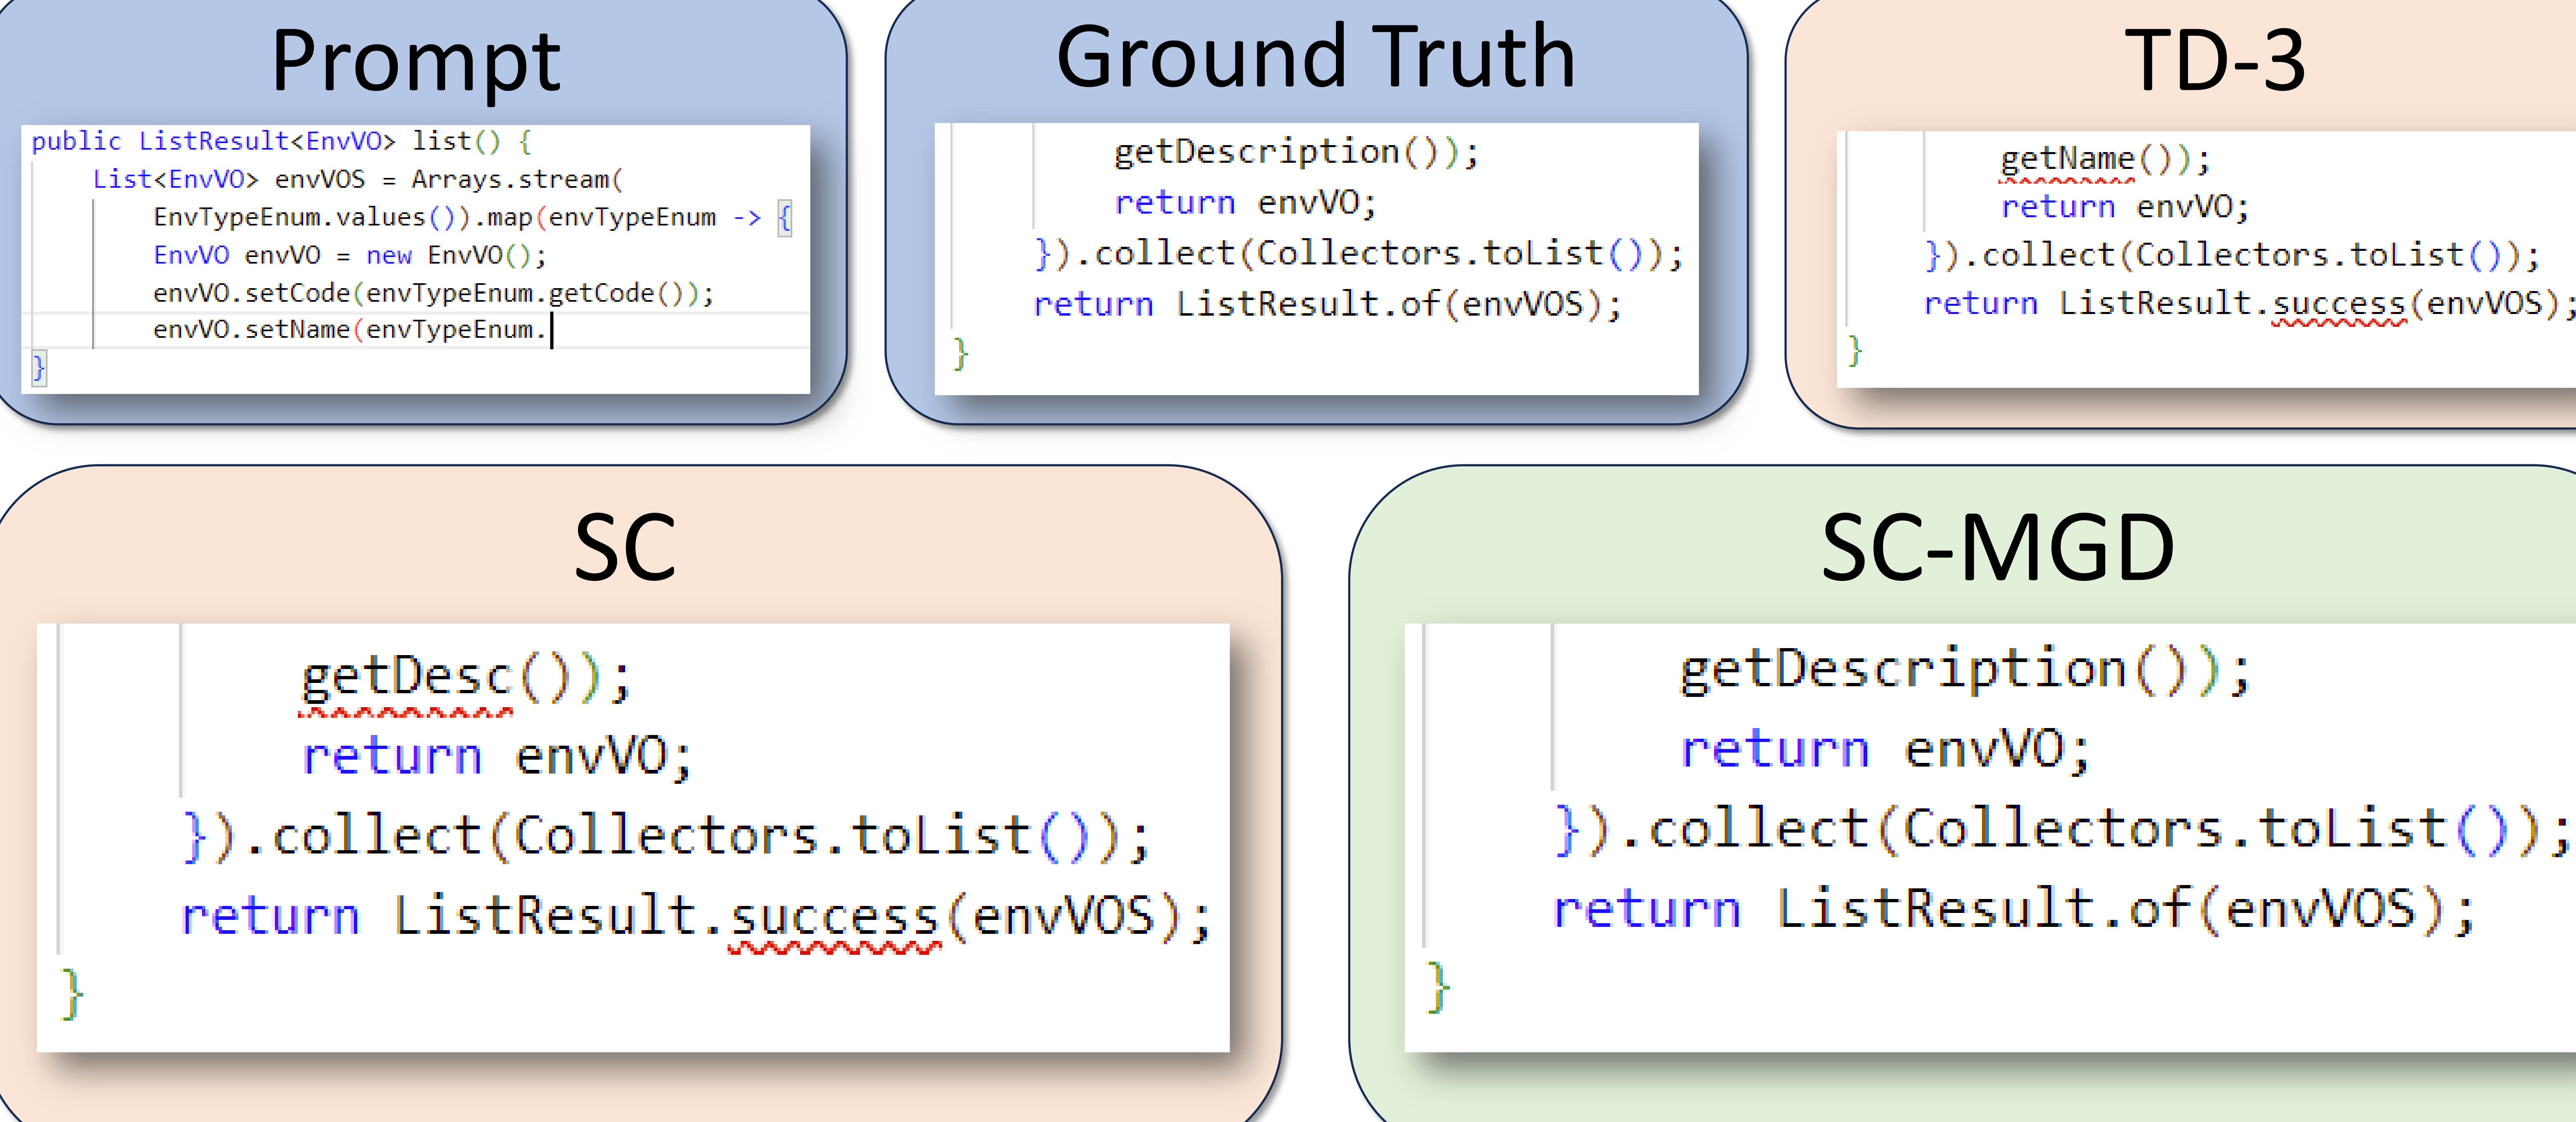
Prompt
public ListResult<EnvVO> list() {
List<EnvVO> envVOS = Arrays.stream(
EnvTypeEnum.values()).map(envTypeEnum -> {
EnvVO envVO = new EnvVO();
envVO.setCode(envTypeEnum.getCode());
envVO.setName(envTypeEnum.
}
Ground Truth
getDescription());
return envVO;
}).collect(Collectors.toList());
return ListResult.of(envVOS);
}
TD-3
getName());
return envVO;
}).collect(Collectors.toList());
return ListResult.success(envVOS);
}
SC
getDesc());
return envVO;
}).collect(Collectors.toList());
return ListResult.success(envVOS);
}
SC-MGD
getDescription());
return envVO;
}).collect(Collectors.toList());
return ListResult.of(envVOS);
}

# Main Content

## TD-3

```java
            getName());
            return envVO;
        }).collect(Collectors.toList());
        return ListResult.success(envVOS);
}
```

## SC

```java
            getDesc());
            return envVO;
        }).collect(Collectors.toList());
        return ListResult.success(envVOS);
}
```

## SC-MGD

```java
            getDescription());
            return envVO;
        }).collect(Collectors.toList());
        return ListResult.of(envVOS);
}
```

## Prompt

```java
public ListResult<EnvVO> list() {
    List<EnvVO> envVOS = Arrays.stream(
        EnvTypeEnum.values()).map(envTypeEnum -> {
        EnvVO envVO = new EnvVO();
        envVO.setCode(envTypeEnum.getCode());
        envVO.setName(envTypeEnum.
}
```

## Ground Truth

```java
            getDescription());
            return envVO;
        }).collect(Collectors.toList());
        return ListResult.of(envVOS);
}
```

## Prompt

```java
@Override
public boolean isModified() {
  var advancedSettings = AdvancedSettingsState.getInstance();
  return !advancedSettingsComponent.getProxyType().equals(advancedSettings.proxyType) ||
      !advancedSettingsComponent.getProxyHost().equals(advancedSettings.proxyHost) ||
      advancedSettingsComponent.getProxyPort() != advancedSettings.proxyPort ||
      advancedSettingsComponent.isProxyAuthSelected() != advancedSettings.isProxyAuthSelected ||
      !advancedSettingsComponent.
}
```

## Ground Truth

```java
      getProxyAuthUsername().equals(advancedSettings.proxyUsername) ||
      !advancedSettingsComponent.getProxyAuthPassword().equals(advancedSettings.proxyPassword);
}
```

## TD-3

```java
      getProxyUser().equals(advancedSettings.proxyUser) ||
      !advancedSettingsComponent.getProxyPassword().equals(advancedSettings.proxyPassword);
}
```

## SC

```java
      getProxyUserName().equals(advancedSettings.proxyUserName) ||
      !advancedSettingsComponent.getProxyPassword().equals(advancedSettings.proxyPassword);
}
```

## SC-MGD

```java
      getProxyAuthUsername().equals(advancedSettings.proxyUsername) ||
      !advancedSettingsComponent.getProxyAuthPassword().equals(advancedSettings.proxyPassword);
}
```

## Prompt

```
public String sendSignedRequest(String baseUrl, String urlPath, LinkedHashMap<String, Object> parameters,
                                HttpMethod httpMethod, boolean showLimitUsage) {
    if (null == secretKey || secretKey.isEmpty() || null == apiKey || apiKey.isEmpty()) {
        throw new BinanceConnectorException(fullErrMsg:"[RequestHandler] Secret key/API key cannot be null or empty!");
    }
    parameters.put(key:"timestamp", UrlBuilder.buildTimestamp());
    String queryString = UrlBuilder.joinQueryParameters(parameters);
    String signature = SignatureGenerator.
}
```

## Ground Truth

```
    getSignature(queryString, secretKey);
    return sendApiRequest(baseUrl, urlPath, signature, parameters,
        httpMethod, RequestType.SIGNED, showLimitUsage);
}
```

## TD-3

```
    generateSignature(queryString, secretKey);
    return sendApiRequest(baseUrl, urlPath, signature, parameters,
        httpMethod, RequestType.SIGNED, showLimitUsage);
}
```

## SC

```
    getBinarySignature(urlPath, queryString, secretKey);
    return sendApiRequest(baseUrl, urlPath, signature, parameters,
        httpMethod, RequestType.SIGNED, showLimitUsage);
}
```

## SC-MGD

```
    getSignature(queryString, secretKey);
    return sendApiRequest(baseUrl, urlPath, signature, parameters,
        httpMethod, RequestType.SIGNED, showLimitUsage);
}
```

## SC-classExprTypes

```
    generateSignature(httpMethod, baseUrl, urlPath, queryString, secretKey);
    return sendApiRequest(baseUrl, urlPath, signature, parameters,
        httpMethod, RequestType.SIGNED, showLimitUsage);
}
```

## SC-classExprTypes-MGD

```
    getSignature(queryString, secretKey);
    return sendApiRequest(baseUrl, urlPath, signature, parameters,
        httpMethod, RequestType.SIGNED, showLimitUsage);
}
```

## Prompt

```
public boolean requestPush(String baseUrl, ZolaMessage message) {
    Request request = new Builder()
            .url(baseUrl + "/api/messages")
            .post(RequestBody.create(ZolaJsonSerializer
            .getInstance().serialize(message), JSON))
            .build();
    Call call = http.newCall(request);
    try (Response response = call.execute()){
        validateResponse(response.code(), message.
}
```

## Ground Truth

```
        getQueueNameValue());
        return true;
    } catch (Exception e) {
        e.printStackTrace();
        throw new ZolaServerConnectionFailedException(
    message:"unexpected exception occurred while communicate with zola messaging server");
    }
}
```

## TD-3

```
        getId());
        return true;
    } catch (Exception e) {
        e.printStackTrace();
        return false;
    }
}
```

## SC

```
        getId());
        return true;
    } catch (Exception e){
        throw new RuntimeException("Can't send push to " + baseUrl, e);
    }
}
```

## SC-MGD

```
        getQueueNameValue());
        return true;
    } catch (Exception e) {
        e.printStackTrace();
        return false;
    }
}
```

## SC-FIM

```
        getQueueName());
        return true;
    } catch (Exception e) {
        e.printStackTrace();
        throw new ZolaServerConnectionFailedException(
    message:"unexpected exception occurred while communicate with zola messaging server");
    }
}
```

## SC-FIM-MGD

```
        getQueueNameValue());
        return true;
    } catch (Exception e) {
        e.printStackTrace();
        throw new ZolaServerConnectionFailedException(
    message:"unexpected exception occurred while communicate with zola messaging server");
    }
}
```

## Prompt

```
@Override
public Page<WorkflowInstanceDTO> list(WorkflowInstanceListParam param) {
    Page<WorkflowInstance> page = new Page<>(param.getCurrent(), param.getPageSize());
    Page<WorkflowInstanceVO> workflowInstancePage = workflowInstanceMapper
        .list(page, param.getWorkflowDefinitionId(), param.getState());
    Page<WorkflowInstanceDTO> result = new Page<>(workflowInstancePage
    .getCurrent(), workflowInstancePage.getSize(), workflowInstancePage.getTotal());
    List<WorkflowInstanceDTO> workflowDefinitionDTOS = WorkflowInstanceVOConvert.INSTANCE.
}
```

## Ground Truth

```
    toDto(workflowInstancePage.getRecords());
    result.setRecords(workflowDefinitionDTOS);
    return result;
}
```

## TD-3

```
    list(workflowInstancePage.getRecords());
    result.setRecords(workflowDefinitionDTOS);
    return result;
}
```

## SC

```
    toDTOList(workflowInstancePage.getRecords());
    result.setRecords(workflowDefinitionDTOS);
    return result;
}
```

## SC-MGD

```
    toDto(workflowInstancePage.getRecords());
    result.setRecords(workflowDefinitionDTOS);
    return result;
}
```

## SC-RLPG

```
    toDtos(workflowInstancePage.getRecords());
    result.setRecords(workflowDefinitionDTOS);
    return result;
}
```

## SC-RLPG-MGD

```
    toDto(workflowInstancePage.getRecords());
    result.setRecords(workflowDefinitionDTOS);
    return result;
}
```

**Prompt**

```java
@Override
public BankAccount findRequired(AccountNumber accountNumber) {
    var optionalBankAccount = find(accountNumber);

    if (optionalBankAccount.isEmpty()) {
        throw new ValidationException(ValidationMessages.
}
```

**Ground Truth**

```java
            ACCOUNT_NUMBER_NOT_EXIST);
    }

    return optionalBankAccount.get();
}
```

**TD-3**

```java
            ACCOUNT_NOT_FOUND);
    }

    return optionalBankAccount.get();
}
```

**SC**

```java
            ACCOUNT_NOT_FOUND);
    }

    return optionalBankAccount.get();
}
```

**SC-MGD**

```java
            ACCOUNT_NUMBER_NOT_EXIST);
    }

    return optionalBankAccount.get();
}
```

**SC-classExprTypes**

```java
            ACCOUNT_NUMBER_EMPTY);
    }

    return optionalBankAccount.get();
}
```

**SC-classExprTypes-MGD**

```java
            ACCOUNT_NUMBER_NOT_EXIST);
    }

    return optionalBankAccount.get();
}
```

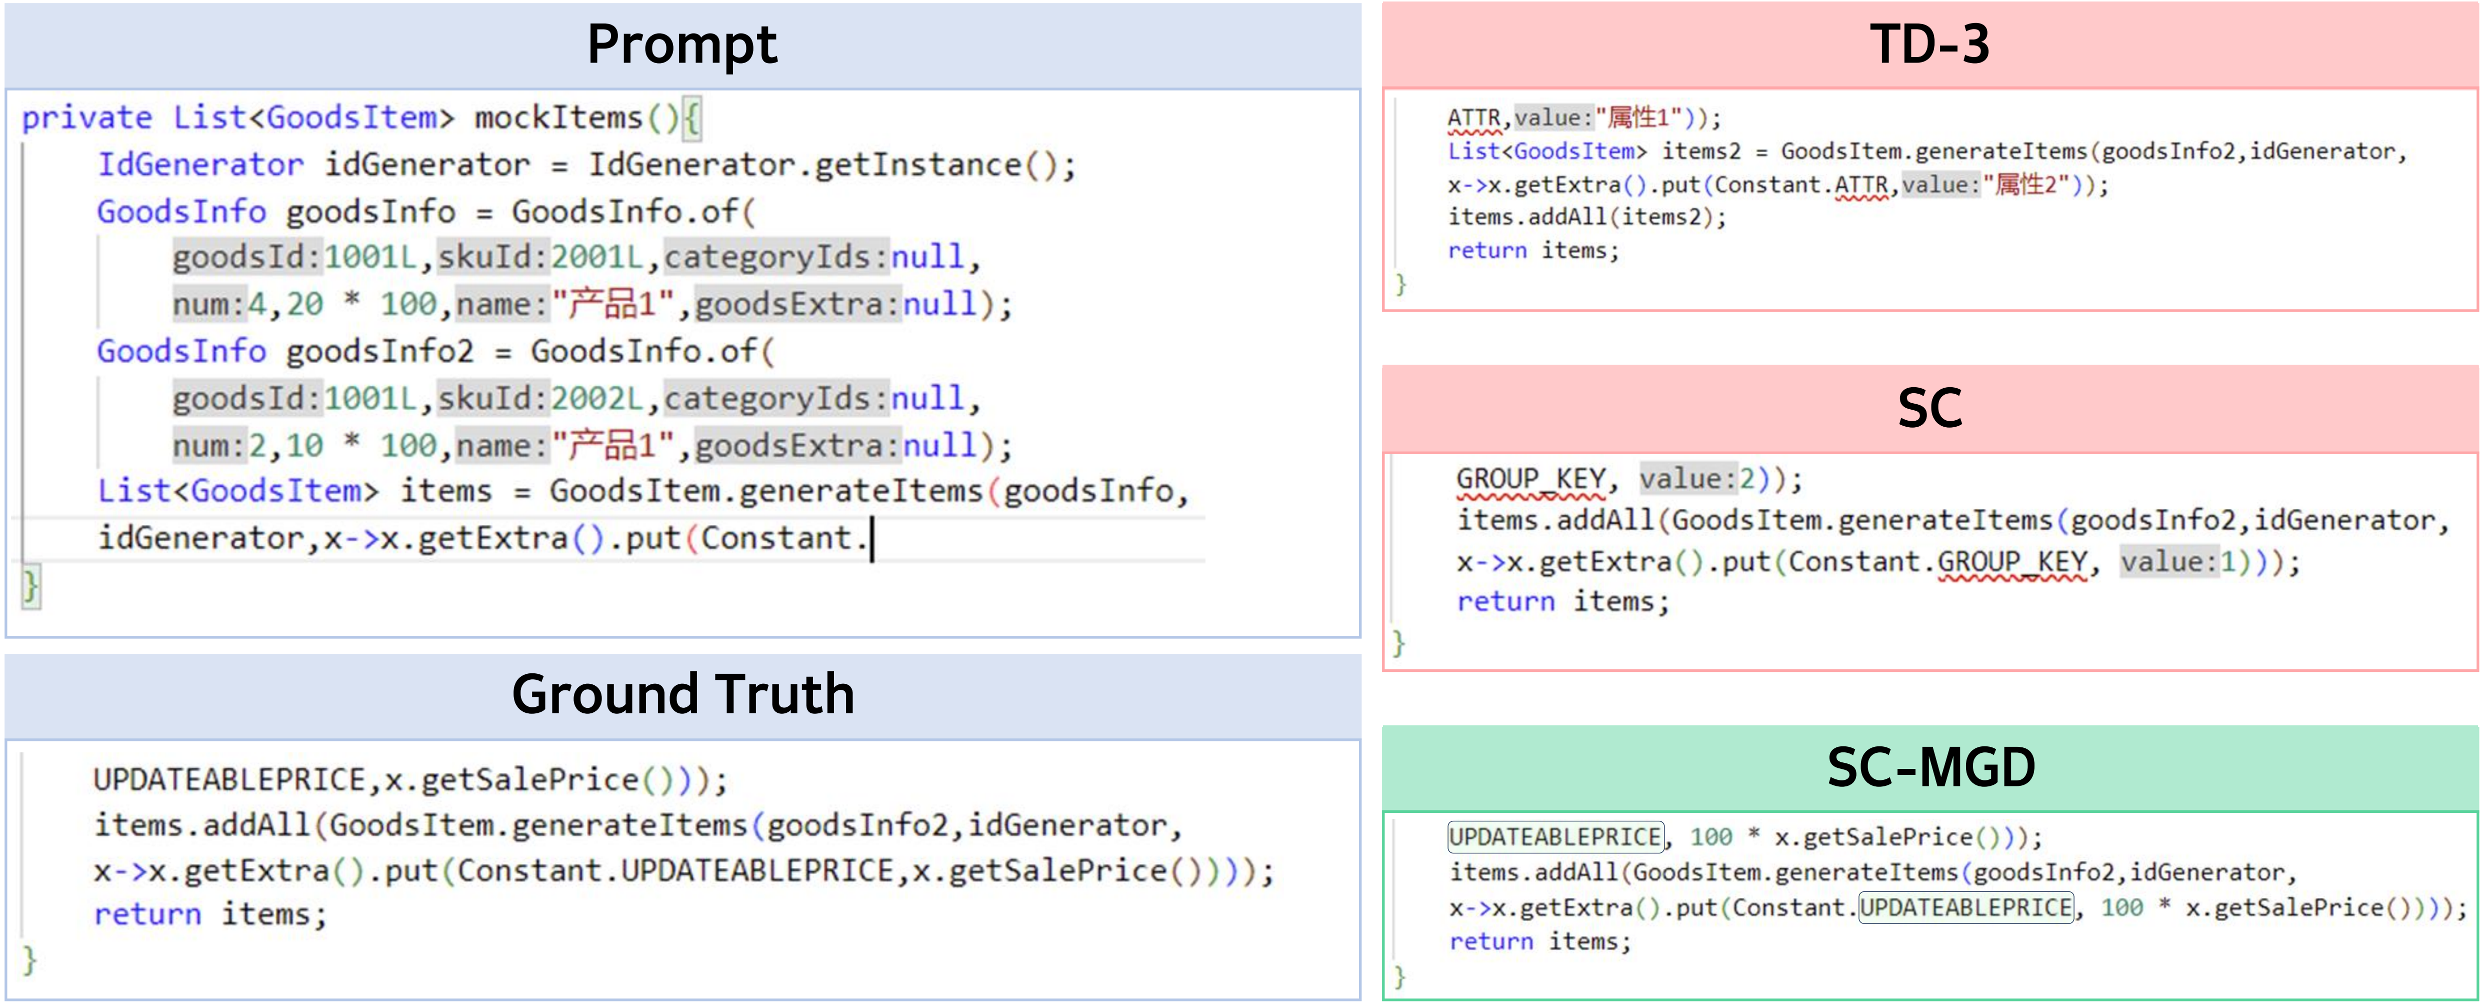
Prompt
private List<GoodsItem> mockItems(){
IdGenerator idGenerator = IdGenerator.getInstance();
GoodsInfo goodsInfo = GoodsInfo.of(
goodsId:1001L,skuId:2001L,categoryIds:null,
num:4,20 * 100,name:"产品1",goodsExtra:null);
GoodsInfo goodsInfo2 = GoodsInfo.of(
goodsId:1001L,skuId:2002L,categoryIds:null,
num:2,10 * 100,name:"产品1",goodsExtra:null);
List<GoodsItem> items = GoodsItem.generateItems(goodsInfo,
idGenerator,x->x.getExtra().put(Constant.
}
Ground Truth
UPDATEABLEPRICE,x.getSalePrice()));
items.addAll(GoodsItem.generateItems(goodsInfo2,idGenerator,
x->x.getExtra().put(Constant.UPDATEABLEPRICE,x.getSalePrice())));
return items;
}
TD-3
ATTR,value:"属性1"));
List<GoodsItem> items2 = GoodsItem.generateItems(goodsInfo2,idGenerator,
x->x.getExtra().put(Constant.ATTR,value:"属性2"));
items.addAll(items2);
return items;
}
SC
GROUP_KEY, value:2));
items.addAll(GoodsItem.generateItems(goodsInfo2,idGenerator,
x->x.getExtra().put(Constant.GROUP_KEY, value:1)));
return items;
}
SC-MGD
UPDATEABLEPRICE, 100 * x.getSalePrice()));
items.addAll(GoodsItem.generateItems(goodsInfo2,idGenerator,
x->x.getExtra().put(Constant.UPDATEABLEPRICE, 100 * x.getSalePrice())));
return items;
}

# Content over

# Example 6

## Prompt

```
public OpenAccountResponse handle(OpenAccountRequest request) {
    var nationalIdentityNumber = request.getNationalIdentityNumber();
    var accountHolderName = getAccountHolderName(request);
    var balance = getBalance(request);

    var timestamp = dateTimeService.now();

    var isBlacklisted = customerGateway.isBlacklisted(nationalIdentityNumber);

    if(isBlacklisted) {
        throw new ValidationException(ValidationMessages.NATIONAL_IDENTITY_NUMBER_BLACKLISTED);
    }

    var bankAccount = createBankAccount(nationalIdentityNumber, accountHolderName, balance, timestamp);

    // TODO: VC: Value object for national identity number
    var exists = nationalIdentityGateway.exists(nationalIdentityNumber);
    if(!exists) {
        throw new ValidationException(ValidationMessages.NATIONAL_IDENTITY_NUMBER_NONEXISTENT);
    }

    bankAccountRepository.add(bankAccount);

    var accountOpened = getAccountOpened(bankAccount, timestamp);
    eventPublisher.
}
```

## Ground Truth

```
    publishEvent(accountOpened);

    return getResponse(bankAccount);
}
```

## TD-3

```
    publish(accountOpened);

    return new OpenAccountResponse(bankAccount.getId());
}
```

## SC

```
    publishEvent(accountOpened);

    return new OpenAccountResponse(bankAccount);
}
```

## SC-MGD

```
    publishEvent(accountOpened);
    return new OpenAccountResponse(bankAccount.getAccountHolderN
                bankAccount.getAccountId());
}
```

## SC-RLPG

```
    publish(accountOpened);

    return getResponse(bankAccount);
}
```

## SC-RLPG-MGD

```
    publishEvent(accountOpened);

    return getResponse(bankAccount);
}
```

# Example 8

## Prompt

```
/**
 * 解析数据输入表名称，同时将表的读取流打开准备读取数据
 * <p>
 * Parse the data input table name, and open the read stream of the table to read the data
 *
 * @param tableName 数据表名称 注意 表格式为: "xxx.NameManager.xxx" 将会被视为NameManager,
 * 直接采取API的setInFilePath的设置参数
 *                  <p>
 *                  Data table name Note that the table format is: "xxx.NameManager.xxx"
 *  will be regarded as NameManager, directly take the setting parameters of API's setInFilePath
 * @return 数据库表的read组件
 * <p>
 * read component of database table
 * @throws IOException 操作流打开异常
 *                     <p>
 *                     Operation stream open exception
 */
@Override
public Reader readStream(String tableName) throws IOException {
    boolean isNameManager = tableName.split(regex:"\\.")[1].equalsIgnoreCase(anotherString:"nameManager");
    try {
        return DataBaseReader.
}
```

## Ground Truth

```
        builder().setConnection(connection).select(this.Schemas).from(isNameManager ? tableName : toSQLTable(tableName)
        ).where(isNameManager ? "" : where);
    } catch (ZHAOLackOfInformation n) {
        n.printStackTrace(System.err);
        throw new ZHAOLackOfInformation(
            "算法库中的数据库读取操作流有尝试被启用，但是启用失败，可能是由于您的API调用异常，本操作流也是需要强转进行参数设置的。" +
            "\n示例：((DataBaseStream) RW.getDT_UDF_Stream(DT_builtIn_UDF.SQLDB_TEXT)).setConnection(连接对象).where(\"sex = '男'\").readStream(s);" + n);
```

## TD-3

```
        of(connection, toSQLTable(tableName), where).setSchemas(Schemas).setNameManager(isNameManager).build();
    } catch (SQLException e) {
        throw new IOException(e);
    }
}
```

## SC

```
        getInstance(connection, toSQLTable(tableName), Schemas, where, isNameManager);
    } catch (SQLException e) {
        e.printStackTrace();
    }
    return null;
}
```

## SC-MGD

```
        builder().setConnection(connection)
                .setInputStream(connection.prepareStatement(isNameManager ? "select * from " +
                    toSQLTable(tableName) + " where " + where : "select * from " + toSQLTable(tableName)))
                .setSchemas(Schemas)
                .setWhere(where)
                .execute();
    } catch (Exception e) {
        logger1.error(msg:"数据读取异常，请检查数据表是否存在，以及数据表的读取权限是否正确：", e);
        throw new IOException(e);
    }
}
```
